# Supplementary material for: Spectral stability of V2 centres in sub-micron 4H-SiC membranes
Source: arXiv:2310.12617 ancillary file (2024-05-13)
Supplement: Supplementary file 1 [file V2_Membrane_Paper_Supplementary.pdf]

# Supplementary materials to:
# Spectral stability of V2-centres in sub-micron 4H-SiC membranes

Jonah Heiler,[1,*] Jonathan Körber,[2,*] Erik Hesselmeier,[2,*] Pierre Kuna,[2] Rainer Stöhr,[2] Philipp Fuchs,[3] Misagh Ghezellou,[4] Jawad Ul-Hassan,[4] Wolfgang Knolle,[5] Christoph Becher,[3] Florian Kaiser,[2,6] and Jörg Wrachtrup[2,7]

[1] *3rd Institute of Physics, University of Stuttgart, 70569 Stuttgart, Germany.*
[2] *3rd Institute of Physics, University of Stuttgart, Pfaffenwaldring 57, 70569 Stuttgart, Germany.*
[3] *Universität des Saarlandes, Fachrichtung Physik, Campus E2.6, 66123 Saarbrücken, Germany.*
[4] *Department of Physics, Chemistry and Biology, Linköping University, 581 83 Linköping, Sweden.*
[5] *Department of Sensoric Surfaces and Functional Interfaces, Leibniz-Institute of Surface Engineering (IOM), Leipzig, Germany.*
[6] *Materials Research and Technology (MRT) Department, Luxembourg Institute of Science and Technology (LIST), 4422 Belvaux, Luxembourg.*
[7] *Max Planck Institute for Solid State Research, Stuttgart, Germany.*

(Dated: October 19, 2023)

## S1. HOME-BUILT WLI-SETUP

To measure the thickness of the membranes in between the final etching steps in the nm-range we made use of the interference of a broadband light source reflected from the thin membranes. As shown in figure S1 (a), our setup consists of a thermal light source, focused through an objective onto our sample. The sample is placed on an xyz-stage for focusing and lateral positioning. The reflected light is sent to a spectrometer, where we record the wavelength-dependent intensity. The reflection from a thin film with refractive index $n_2$ and thickness $t$ at perpendicular incidence

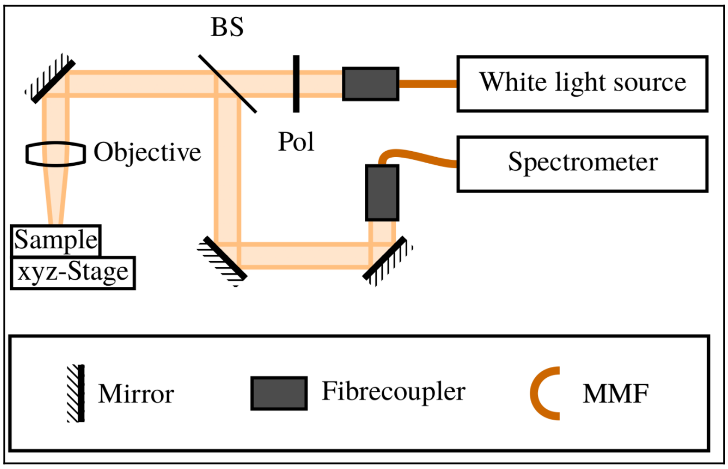


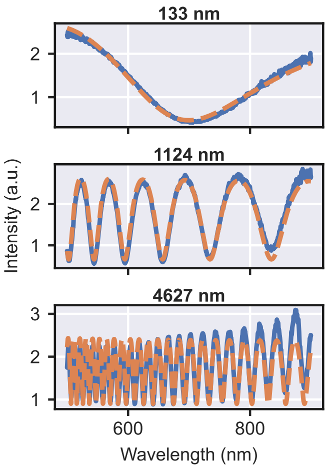


**Figure S1: Home-built WLI setup and example measurements. (a)** Schematic of the WLI setup. Collimated light from a thermal light source (*Thorlabs SLS201L*) is focussed through an objective (NA 0.4) onto the membrane sample. The reflected light is guided onto a broadband spectrometer (*Lasertack LR2,* 200–1200 nm) to record the thin-film interference. **(b)** Recorded interference on three different membranes (blue curves). The thickness shown above each plot is acquired with a fit (orange, dashed line).

---

[*] These authors contributed equally to this work

can be expressed as [1]

$$R(t) = \frac{r_{12}^2 + r_{23}^2 + r_{12}r_{23}\cos(\delta)}{1 + (r_{12}r_{23})^2 + r_{12}r_{23}\cos(\delta)} \quad (1)$$

with the thickness-dependent phase shift $\delta = 4\pi n_2 t/\lambda$ and the Fresnel coefficients for reflection

$$r_{ij} = \frac{n_i - n_j}{n_i + n_j}. \quad (2)$$

In our case the membrane is surrounded by air, i.e., the refractive indices above and below the sample, $n_1$ and $n_3$, are $\sim 1$. For the refractive index of 4H-SiC we use the Sellmeier parameters from [2]. To extract the thickness from a measurement, we divide the raw measurement by a reference measurement on a silver mirror (*Thorlabs PF10-03-P01*) to correct it for the spectrum of the light source and all the optics and consecutively fit it with the function

$$f(t) = a \cdot R(t) + b. \quad (3)$$

As shown in the three examples in figure S1 (b) this method yields good fit results and enables us to measure the thickness in the desired range from 100 nm up to several µm. Smaller fit deviations on the envelope of the signal, as they can be seen in the lower example of figure S1 (b), typically arise from a non-perfect reference measurement, which is slightly affected by the focus position. Since they do not influence the thickness dependent part of the fit function, we do not expect them to significantly influence our thickness results.

## S2. FINAL MEMBRANE THICKNESSES

After all fabrication steps of the main sample, also including the $SF_6$ soft-ICP etching step, we measured the thickness at the position of minimum thickness of each membrane. When moving the beam of the home-built WLI across a sample with varying thickness, the visible fringes shift their spectral position. Here, a shift towards higher wavelengths indicates an increase of the thickness and a shift towards lower wavelengths a thickness decrease. Since the signal strength in our setup is high enough, we can use integration times of 50–200 ms at the spectrometer and thus record the shift of fringes while moving the position in real-time. We make use of this fact to find the position of minimum thickness for each membrane by laterally moving the beam to a position where any addditional, lateral movement shifts the fringes to higher wavelengths.

The left part of table S1 shows the measured thickness for all 12 membranes at their respective minimum position. To get a feeling for the stability of our thickness measurements, i.e. how reproducible one can find the minimum thickness position and how strongly the fitted values for the same membrane deviate, we decided to measure the membranes a second time. This time, we flipped the sample in our setup by 90°. Since 4H-SiC is a birefringent material it exhibits an extraordinary refractive index $n_e$ for polarization parallel to the crystal c-axis and an ordinary refractive index $n_o$ for polarization perpendicular to the c-axis with $n_o > n_e$ [3, 4]. In the original sample orientation, the polarization of our white light source was adjusted parallel to the ordinary index by using a wire grid polarizer. With the sample flipped, we changed the polarization to be perpendicular to the crystal c-axis and recorded all fringes at the positions of minimum thickness slightly shifted to lower wavelengths, as expected due to the lower refractive index for this orientation. The right part of table S1 displays our fitted results of the flipped measurements, taking the different refractive index into account. Indeed the values almost perfectly fit the ones acquired with the original sample orientation, thus showing the stability and reproducibility of our thickness measurements. As we find a maximum deviation of 5 nm between the two measurements for membrane D3, we estimated an accuracy of 10 nm for the thickness values given in the main manuscript.

For an estimate of the thickness variation in the central part of each membrane we measured the thickness 50 µm left, above, right and below the position of minimum thickness in addition. The results are displayed in figure S2 together with images of each membrane, acquired by an optical profiler. For the membranes of D1-D3 the measurement 50 µm left of the center was not possible, since the thickness gradient already became to steep for an evaluable result from our WLI. Overall, our measurements show thickness variations in the range of 50–120 nm for the inner parts of the membranes.

To check how much material we removed at the $SF_6$ soft-ICP etching step after the post-fabrication annealing we also measured the thickness of each membrane before this step. As expected, there was only a slight material

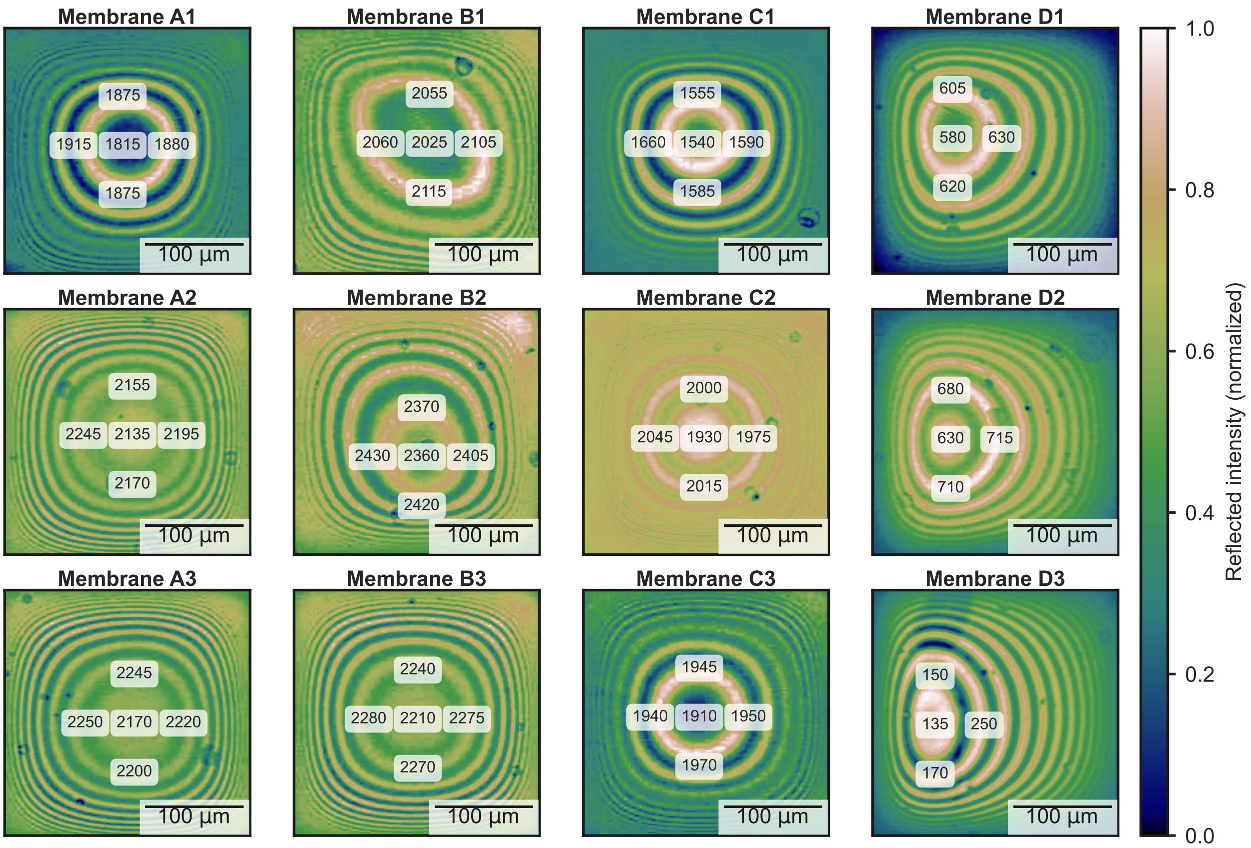


**Figure S2: Single wavelength interference and measured thickness of the different membranes.** Reflection of the different membranes with laser light ($\lambda = 532$ nm), measured with an optical profiler (*Bruker ContourX*). Thickness variations of the membranes lead to different interference for the fixed laser wavelength and thus creates fringes in reflection. The numbers in the boxes show thicknesses in nm, measured with the home-built WLI, for the center of the membranes and positions shifted by 50 µm from the central position to the left, top, right and bottom, respectively.

removal of ∼30 nm at this step. We assume that the increased roughness after this step that we report in the main manuscript results from this removal with the contamination that lead to an increased background fluorescence acting as an etching mask.

**Table S1:** Measured thickness with the light source polarized parallel (left) and antiparallel (right) to the crystal c-axis

| | **1** | **2** | **3** |
|---|---|---|---|
| **A** | 1816 nm | 2134 nm | 2169 nm |
| **B** | 2025 nm | 2358 nm | 2211 nm |
| **C** | 1541 nm | 1929 nm | 1908 nm |
| **D** | 578 nm | 631 nm | 133 nm |

| | **1** | **2** | **3** |
|---|---|---|---|
| **A** | 1817 nm | 2135 nm | 2170 nm |
| **B** | 2021 nm | 2361 nm | 2211 nm |
| **C** | 1543 nm | 1928 nm | 1908 nm |
| **D** | 577 nm | 631 nm | 128 nm |

## S3. ROUGHNESS AFTER FABRICATION

To characterize the surface quality of our fabrication processes we investigated the surface topography of a sample from the same batch than the main sample after the polishing processes and a second time after the reactive-ion-

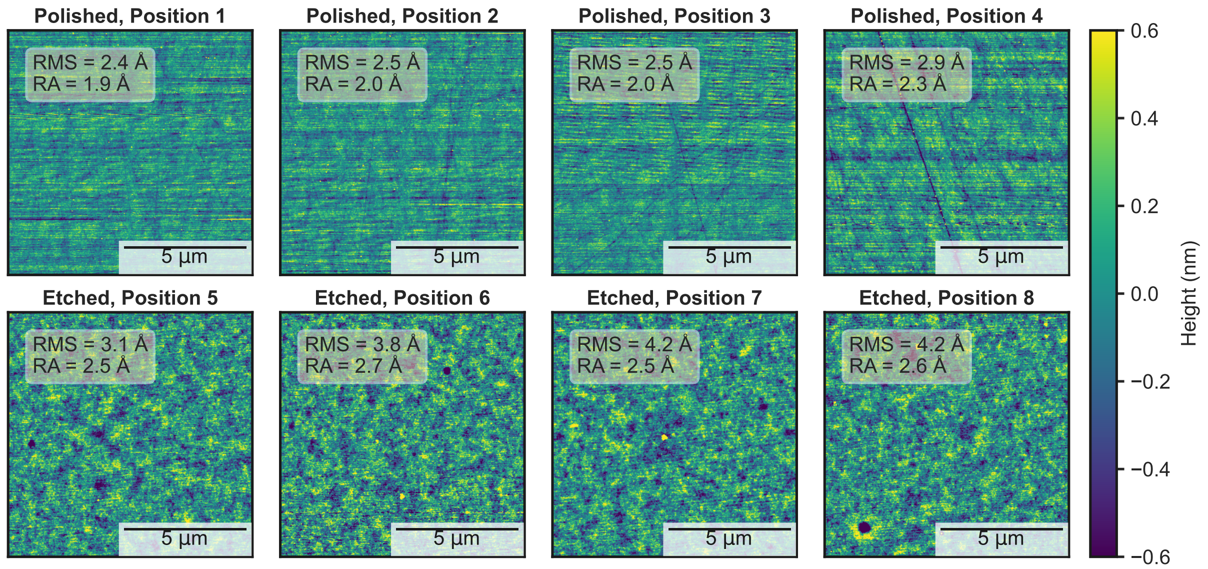


**Figure S3: Surface topography of a reference sample after fabrication.** Topography of a reference sample from the same batch than the main sample of the manuscript after the final polishing step (upper row) and a 40 µm-deep etching (lower row). The measurements were taken for each four arbitrary positions on the sample with an commercial AFM (*Veeco Dimension Icon, Veeco Instruments*).

etching. Each time, we measured the surface roughness with an AFM on four arbitrary positions on the sample. During the course of our measurements, the damping of the optical table of the AFM was not operationable which lead to an increased noise. This is visible in a periodic series of thin lines in all scans. We thus conclude that the given roughness ranges are an upper limit of the real surface roughness of the sample.

As shown in the upper row of figure S3, after the final polishing the surface shows an RMS-roughness of 2.4–2.9 Å with a few shallow scratches remaining from the diamond abrasives still visible. These scratches completely disappear after etching for 40 µm, which can be seen in the lower panel of figure S3. The final surface roughness after etching is in the range of 3.1–4.2 Å, i.e. slightly increased compared to the results after polishing. This can be mainly explained by the appearance of small etch pits resulting from the long etching process, that can be a few nm deep and thus increase the RMS value.

## S4. REPRODUCIBILITY OF THE MEMBRANE FABRICATION

To show the reproducibility of our presented fabrication recipe, we repeated it several times on different samples. As displayed in figure S4 for two different samples, the surface roughness after polishing and after deep RIE turns out to be similar than our results for the sample of the main manuscript. Again, we see shallow scratches after our final polishing step, that completely vanish after etching for a few 10 µm and the final rms-roughness after the etching is within a range of 3.1–3.8 Å. Figure S4 (c) shows microscope images of sub-µm membranes from each a different sample. As for the membranes of the main sample, thicknesses of only a few 100 nm thickness (here even below 100 nm) can be achieved with a region of homogeneous thickness in the central part.

## S5. ADDITIONAL MEMBRANE SPECTRA

We have measured additional spectra in membrane D2 before and in membrane D3 after the post-fabrication. An analogous representation to Figure 2 in the main text of this data is depicted in Figure S5. It shows the same trend that the number of V1- and V2-centres increases with the post-processing step, while the number of unidentified peaks decreases.

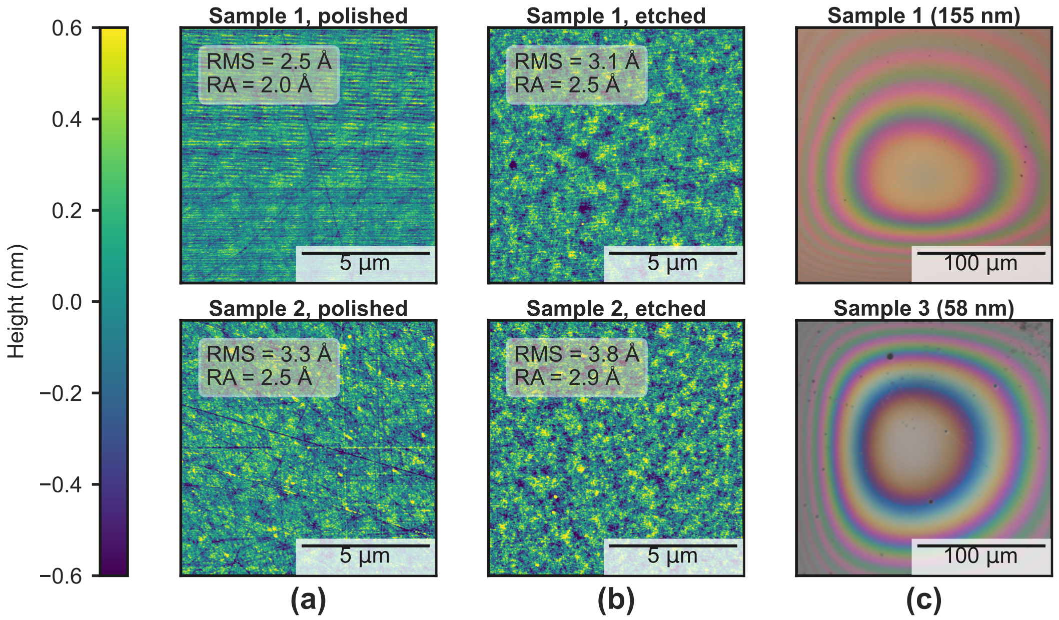


**Figure S4: Additional membrane samples fabricated with the recipe presented in the main manuscript. (a)** AFM surface topography of two different samples after thinning and polishing of the wafer side. **(b)** AFM surface topography of the two samples from (a) after subsequent RIE with the same process as in the main manuscript and a removal of several µm. **(c)** Microscope images of two arbitrary membranes from two different samples. The minimum thickness, measured by our home-built WLI, is given in the respective title.

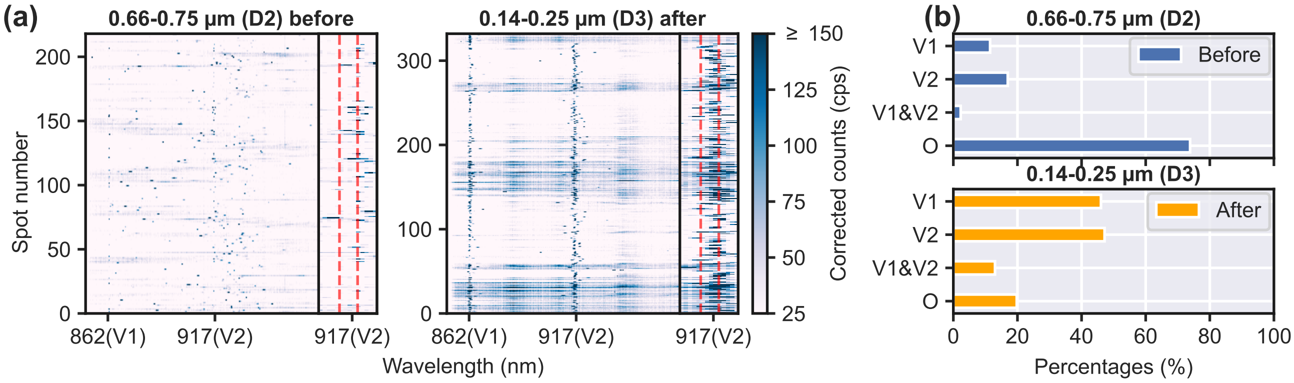


**Figure S5: Additional spectra statistics before and after post-processing. (a)** Stacked photoluminescence spectra from different spots in membranes D2 and D3 before and after the post fabrication processing, respectively. **(b)** Percentages of V1 peaks, V2 peaks, both V1 and V2 peaks (V1&V2) and unidentified peaks (O) in the automatically acquired spectra.

## S6. STABLE PLE LINES

In addition to the emitters whose PLE lines we show in Figure 3 of the main text, we have found emitters with more stable PLE lines in membrane D2. As an example, three of these emitters are depicted in Figure S6. Note, that the individual lines of the presented data are not shifted to a fixed position, thus demonstrating the very high spectral stability of the PLE measurements.

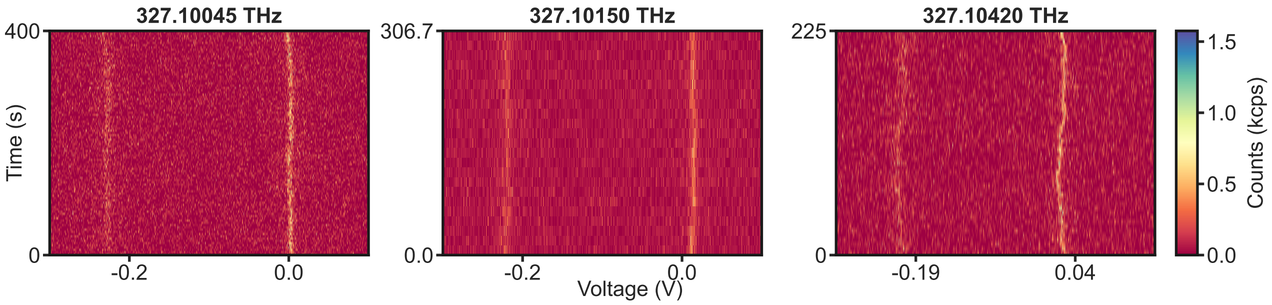


**Figure S6: Stable PLE lines in Membrane D2.** Non-shifted voltage over time PLE scans at 3 nW resonant laser power for three different emitters in membrane D2 (630–715 nm) that show only little spectral wandering.

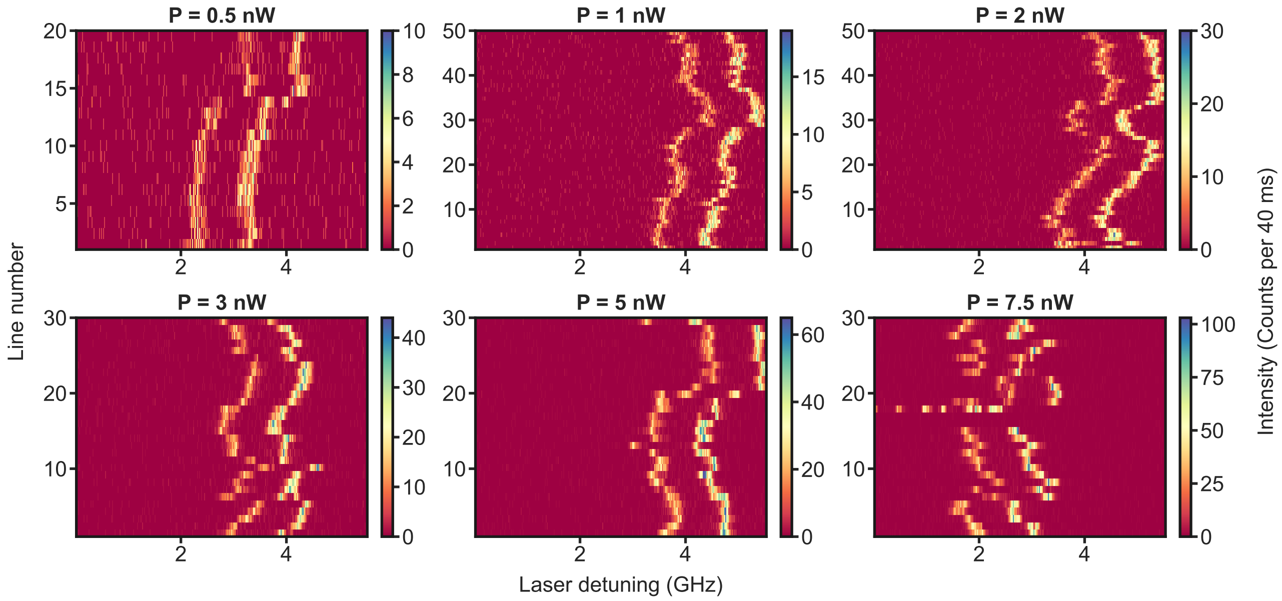


**Figure S7: Multi-line PLE scans in the membrane D3.** In all scans, the integration time per point is 40 ms. From left to right and top to bottom: Data recorded for resonant laser power $P$ = 0.5 nW, $P$ = 1 nW, $P$ = 2 nW, $P$ = 3 nW, $P$ = 5 nW, and $P$ = 7.5 nW.

## S7. PLE LINEWIDTHS IN THE 0.25 µm MEMBRANE D3

In this section, we discuss the experimental data for the measurement of the resonant absorption lines of V2 centres in the thin 0.25 $\mu$m membrane D3. The experimental data in main text Figure 3(d) shows an apparent tendency for reduced linewidths at higher pump powers. In the following, we will show that these observations can be explained by a combination of laser-induced charge state instability, as well as laser-induced spectral jumping of the V2 centre during the laser scans. We mention that we observe these instabilities mainly in the thinnest 0.25 $\mu$m membrane (D3), and, to a significantly lesser extent in the second-thinnest 0.58–0.63 µm membrane (D1). These instabilities prevented us from recording resonant absorption spectra at optical power levels above 7.5 nW (15 nW) for emitters in the membrane D3 (D1). Our subsequent investigations now focus on the measurements in the thinnest membrane D3. Raw data of a single V2 centre on which we performed multi-line PLE scans for resonant pump powers in the range $P$ = 0.5–7.5 nW is shown in Figure S7.

At first glance, it is visible that increased resonant pump powers lead to an increased chance to record more than two resonant absorption lines during one scan. This indicates that spectral jumps occurred during a laser scan. The percentage of line jumps as a function of the laser power is shown in Figure S8(a). We find an increased rate of spectral jumps from $P \geq 3$ nW. For our linewidths analysis, we systematically exclude all PLE scans in which the

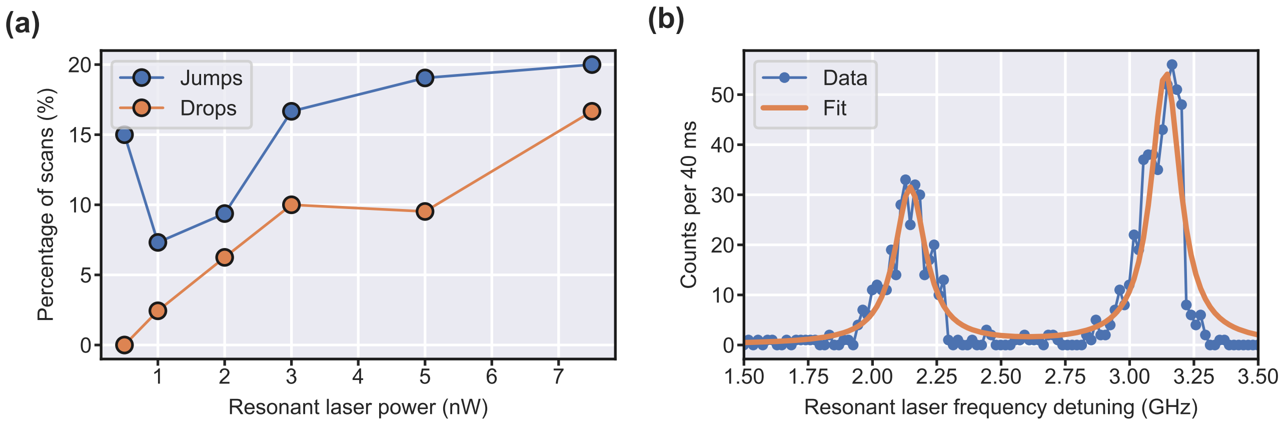


**Figure S8: Spectral jumps and sudden intensity drops during PLE line scans. (a)** Power-dependent percentage of scans in which spectral jumps and sudden intensity drops were observed (cf. also table S2). Lines between markers are a guide to the eye. **(b)** Exemplary data set in which a sudden intensity drop is observed (line 9 of the PLE scan with $P$ = 7.5 nW). The double-Lorentzian fit to the data is non-ideal, especially for the $A_2$ peak.

**Table S2:** Data processing for the PLE scans in the membrane D3. Lines that have been excluded are listed in the columns "Lines with jumps", "Lines too close to edge", and "Lines with no PLE". Fitted scans refers to the number of lines that were summed up to extract the resonant absorption linewidths of the $A_1$ and $A_2$ transitions, respectively.

| Power (nW) | Total scans | Lines with jumps | Lines too close to edge | Lines with no PLE | Lines with potential sudden drops | Used scans | $A_1$ linewidth (MHz) | $A_2$ linewidth (MHz) |
|---|---|---|---|---|---|---|---|---|
| **0.5** | 20 | 4, 11, 14 | | | | 17 | 168 | 187 |
| **1.0** | 50 | 12, 16, 40 | 29, 30, 31, 32, 33, 34, 35, 36, 37 | | 19 | 38 | 140 | 154 |
| **2.0** | 50 | 2, 32, 34 | 21, 22, 24, 25, 35, 36, 37, 38, 39, 40, 41, 42, 43, 44, 45, 46, 47, 48 | | 12, 50 | 29 | 157 | 146 |
| **3.0** | 30 | 1, 6, 10, 18, 27 | | | 17, 26, 29 | 25 | 117 | 116 |
| **5.0** | 30 | 9, 17, 19, 20 | 21, 22, 23, 24, 25, 26, 27, 28, 29 | | 6, 11 | 17 | 133 | 116 |
| **7.5** | 30 | 2, 18, 19, 21, 25, 29 | | 16, 17 | 9, 11, 14, 15, 30 | 22 | 134 | 119 |

number of resonant peaks was greater than 2.

Another observation that we made at increased laser powers is an increased tendency for rapid drops of the fluorescence intensity, e.g., due to charge state ionisation of the emitter during the scan. An exemplary scan is shown in Figure S8(b), where the sudden intensity drop occurs during the scan over the $A_2$ transition. The sudden intensity drop results in an asymmetric line shape, for which the Lorentzian fit delivers an underestimation of the linewidth. As shown in Figure S8(a), the percentage of sudden intensity drops increases steadily with the resonant laser power. However, we also mention here that the low photon detection events at the lower laser powers $P \lesssim 3$ nW make it difficult to faithfully distinguish sudden intensity drops from statistical fluctuations due to photon shot noise. For this reason, we did not attempt to remove PLE scans with sudden intensity drops from the linewidth analysis. However, this also means that our data analysis potentially underestimates linewidths in experimental settings where sudden intensity drops more frequently. We believe that this explains the apparent linewidth decrease in Figure 3(d) of the main text. Considering these insights, we believe that the most accurate values for the $A_1$ and $A_2$ linewidths are

**Table S3:** Linewidths in MHz of different emitters in different regions before the post-fabrication processing. The emitter number refers only to the respective region before post-processing and is used to distinguish PLE series of different emitters in it.

| Region | **Bulk etched (MHz)** | | | | **Bulk polished (MHz)** | | | | | |
|---|---|---|---|---|---|---|---|---|---|---|
| Emitter | 1 | | 2 | | 1 | | 2 | | 3 | |
| Transition | $A_1$ | $A_2$ | $A_1$ | $A_2$ | $A_1$ | $A_2$ | $A_1$ | $A_2$ | $A_1$ | $A_2$ |
| **Power (nW)** | | | | | | | | | | |
| **1.0** | 97.1 | 78.9 | 35.5 | 76.5 | 109.3 | 78.5 | 80.3 | 80.1 | 42.2 | 39.0 |
| **2.0** | 86.1 | 61.1 | 47.4 | 49.6 | 111.5 | 78.0 | 40.8 | 56.6 | 53.3 | 45.6 |
| **3.0** | - | - | 50.1 | 43.6 | - | - | 113.3 | 104.1 | 56.6 | 46.0 |
| **4.0** | 79.5 | 71.7 | 52.8 | 48.5 | 95.4 | 91.6 | - | - | - | - |
| **5.0** | - | - | 62.3 | 45.9 | - | - | 130.8 | 97.5 | 67.0 | 50.6 |
| **6.0** | 102.3 | 75.3 | 58.9 | 49.1 | 101.4 | 90.2 | - | - | - | - |
| **7.5** | - | - | - | - | - | - | 123.0 | 107.9 | 55.3 | 48.6 |
| **8.0** | 115.9 | 70.4 | 53.7 | 55.0 | 116.0 | 94.8 | - | - | - | - |
| **10.0** | 81.7 | 66.3 | 65.1 | 56.7 | 102.2 | 87.5 | - | - | 65.1 | 47.9 |
| **12.0** | - | - | 65.4 | 53.6 | - | - | - | - | - | - |
| **15.0** | 85.0 | 78.2 | 77.4 | 54.8 | 115.6 | 103.1 | - | - | - | - |
| **20.0** | 68.9 | 79.7 | - | - | 105.0 | 85.2 | - | - | - | - |
| **30.0** | 96.3 | 62.1 | - | - | 131.8 | 75.9 | - | - | - | - |

| Region | **D1 (MHz)** | | | | | | | | **D2 (MHz)** | | | | | | | | | |
|---|---|---|---|---|---|---|---|---|---|---|---|---|---|---|---|---|---|---|
| Emitter | 1 | | 2 | | 3 | | 4 | | 1 | | 2 | | 3 | | 4 | | 5 | |
| Transition | $A_1$ | $A_2$ | $A_1$ | $A_2$ | $A_1$ | $A_2$ | $A_1$ | $A_2$ | $A_1$ | $A_2$ | $A_1$ | $A_2$ | $A_1$ | $A_2$ | $A_1$ | $A_2$ | $A_1$ | $A_2$ |
| **Power (nW)** | | | | | | | | | | | | | | | | | | |
| **1.0** | - | - | - | - | - | - | - | - | - | - | - | - | 29.3 | 18.7 | 9.1 | 17.2 | 8.2 | 5.6 |
| **1.5** | 20.8 | 16.7 | 11.0 | 17.2 | 30.4 | 22.1 | 21.6 | 20.8 | 29.4 | 22.5 | 11.7 | 13.2 | 31.8 | 20.7 | 11.4 | 16.8 | 36.1 | 18.8 |
| **2.0** | 19.5 | 17.5 | 16.6 | 17.1 | 34.6 | 21.0 | 32.4 | 22.5 | 32.8 | 21.7 | 19.5 | 17.3 | 35.6 | 23.2 | 20.7 | 17.3 | 34.9 | 21.0 |
| **2.5** | 27.0 | 19.2 | 15.7 | 18.9 | 36.7 | 23.2 | 40.4 | 21.5 | 33.7 | 22.7 | 22.2 | 16.9 | 39.0 | 24.3 | 21.0 | 12.0 | 40.9 | 21.1 |
| **3.0** | 32.5 | 18.9 | 29.1 | 15.7 | 44.7 | 20.0 | 33.9 | 21.3 | 34.6 | 26.8 | 31.2 | 17.7 | 41.4 | 27.7 | 24.5 | 11.8 | 35.5 | 23.4 |
| **3.5** | 35.4 | 20.3 | 30.0 | 18.7 | 42.9 | 18.2 | 41.5 | 22.2 | - | - | 27.0 | 16.9 | 40.5 | 26.1 | 26.0 | 15.3 | 33.5 | 21.4 |
| **4.0** | 30.2 | 16.5 | 33.6 | 14.1 | 43.3 | 20.8 | 47.6 | 23.6 | 39.1 | 27.7 | - | - | - | - | - | - | - | - |
| **4.5** | - | - | - | - | 41.5 | 22.9 | 46.6 | 24.3 | - | - | - | - | - | - | - | - | - | - |

obtained at $P \sim 1$–$2$ nW, the power levels at which sudden intensity drops occur rather infrequently, while providing a reasonable signal-to-noise for obtaining a good fit quality. At these powers, we measured 140 MHz and 157 MHz for the $A_1$ transition, as well as 154 MHz and 146 MHz for the $A_2$ transition.

In table S2, we show additionally, which PLE scans have been excluded from the linewidth analysis based on the three criteria:

- Number of resonant peaks is greater than 2 (spectral jumps).
- No PLE signal was observed during a scan (0 peaks).
- One optical transition being closer than 0.3 GHz from the start/stop of a laser scan (may result in a lower fit quality).

## S8. ALL EXTRACTED PLE LINEWIDTHS

Tables S3 and S4 show the linewidths extracted as described in the section on resonant laser excitation measurements of the main text. The $A_1$ and $A_2$ linewidths before (after) post-fabrication processing in a certain region for one specific power in Figure 3(d) of the main text are obtained from Table S3 (S4) as the mean value for all emitters measured in the respective region at this power. In the case of membranes C2 and D3, there was only one series measured. Therefore, their linewidth, displayed in Figure 3(d), can be directly found in Table S4.

**Table S4:** Linewidths in MHz of different emitters in different regions after the post-fabrication processing. The emitter number refers only to the respective region after post-processing and is used to distinguish PLE series of different emitters in it.

| Region | **Bulk (MHz)** | | | | | | **C2 (MHz)** | | **D1 (MHz)** | | | | **D3 (MHz)** | |
|---|---|---|---|---|---|---|---|---|---|---|---|---|---|---|
| Emitter | 1 | | 2 | | 3 | | 1 | | 1 | | 2 | | 1 | |
| Transition | $A_1$ | $A_2$ | $A_1$ | $A_2$ | $A_1$ | $A_2$ | $A_1$ | $A_2$ | $A_1$ | $A_2$ | $A_1$ | $A_2$ | $A_1$ | $A_2$ |
| **Power (nW)** | | | | | | | | | | | | | | |
| **0.5** | - | - | - | - | - | - | - | - | - | - | - | - | 167.8 | 186.7 |
| **1.0** | 40.8 | 42.8 | 51.4 | 65.9 | 48.7 | 46.1 | 24.6 | 64.5 | 46.6 | 29.9 | 48.0 | 35.5 | 139.7 | 154.0 |
| **1.5** | - | - | - | - | - | - | - | - | - | - | 58.9 | 38.7 | - | - |
| **2.0** | 59.7 | 54.8 | 66.8 | 79.3 | - | - | 63.5 | 71.3 | 44.5 | 29.1 | 66.0 | 48.7 | 156.5 | 145.5 |
| **2.5** | - | - | - | - | - | - | - | - | - | - | 71.1 | 37.5 | - | - |
| **3.0** | 63.1 | 63.9 | 78.1 | 82.3 | 33.3 | 36.4 | 50.5 | 75.8 | 45.3 | 33.8 | - | - | 117.0 | 115.7 |
| **4.0** | 83.2 | 64.8 | 81.4 | 83.7 | - | - | 87.1 | 76.7 | 46.2 | 31.8 | - | - | - | - |
| **5.0** | 71.6 | 66.0 | 88.5 | 84.4 | 82.2 | 64.7 | 56.5 | 106.5 | 45.0 | 33.6 | 72.3 | 52.5 | 133.0 | 116.2 |
| **7.0** | 76.9 | 67.3 | 89.4 | 89.2 | - | - | 84.3 | 92.3 | 48.2 | 36.9 | - | - | - | - |
| **7.5** | - | - | - | - | - | - | - | - | - | - | - | - | 134.5 | 118.8 |
| **10.0** | 77.4 | 69.2 | 93.7 | 87.9 | 69.2 | 66.8 | 111.4 | 90.4 | 56.8 | 38.5 | 88.5 | 63.3 | - | - |
| **10.0** | 77.4 | 69.2 | 93.7 | 87.9 | 69.2 | 66.8 | 96.6 | 87.0 | 56.8 | 38.5 | 88.5 | 63.3 | - | - |
| **13.0** | - | - | 88.5 | 93.3 | - | - | - | - | - | - | - | - | - | - |
| **14.0** | - | - | - | - | - | - | - | - | 58.7 | 44.6 | - | - | - | - |
| **15.0** | 78.0 | 93.6 | - | - | 79.2 | 69.5 | 117.8 | 138.0 | - | - | - | - | - | - |
| **16.0** | - | - | 86.7 | 91.0 | - | - | - | - | - | - | - | - | - | - |
| **20.0** | 99.0 | 96.6 | 88.6 | 97.9 | 83.9 | 66.4 | 156.0 | 149.2 | - | - | - | - | - | - |
| **20.0** | 99.0 | 96.6 | 88.6 | 97.9 | 83.9 | 66.4 | 102.3 | 134.4 | - | - | - | - | - | - |
| **25.0** | 111.1 | 108.7 | 95.9 | 97.6 | 81.1 | 75.9 | - | - | - | - | - | - | - | - |
| **30.0** | 132.1 | 131.8 | 101.3 | 96.0 | 88.9 | 74.5 | 146.0 | 131.7 | - | - | - | - | - | - |
| **35.0** | 140.0 | 145.7 | 96.0 | 98.9 | 101.4 | 86.5 | - | - | - | - | - | - | - | - |
| **40.0** | 125.6 | 132.5 | - | - | 100.8 | 83.5 | 134.2 | 140.8 | - | - | - | - | - | - |
| **45.0** | - | - | 102.1 | 105.7 | - | - | - | - | - | - | - | - | - | - |
| **50.0** | - | - | - | - | 102.7 | 87.7 | - | - | - | - | - | - | - | - |
| **60.0** | - | - | - | - | 109.4 | 76.7 | 175.1 | 141.4 | - | - | - | - | - | - |
| **70.0** | - | - | - | - | 103.9 | 92.6 | - | - | - | - | - | - | - | - |
| **100.0** | - | - | - | - | 113.5 | 92.7 | - | - | - | - | - | - | - | - |

[1] J. Bae, J. Park, H. Ahn, and J. Jin, Optics Express, Vol. 29, Issue 20, pp. 31615-31631 **29**, 31615 (2021).

[2] S. Wang, M. Zhan, G. Wang, H. Xuan, W. Zhang, C. Liu, C. Xu, Y. Liu, Z. Wei, and X. Chen, Laser & Photonics Reviews **7**, 831 (2013).

[3] M. O. de Vries, S. i. Sato, T. Ohshima, B. C. Gibson, J. M. Bluet, S. Castelletto, B. C. Johnson, and P. Reineck, Advanced Optical Materials **9**, 2100311 (2021).

[4] P. T. B. Shaffer, Applied Optics, Vol. 10, Issue 5, pp. 1034-1036 **10**, 1034 (1971).
